# Supplementary material for: ThermoHands: A Benchmark for 3D Hand Pose Estimation from Egocentric Thermal Images
Source: arXiv:2403.09871 source file (2025-02-27)
Supplement: Supplementary file 1 [file datasheet.tex]

\section{Datasheet for Datasets}
We follow the guidelines of the datasheets for datasets~\cite{gebru2021datasheets} to explain the motivation, composition, collection,
recommended use case, and other details of the ThermoHands dataset.

\subsection{Motivation}

\noindent\textbf{For what purpose was the dataset created?}

ThermoHands was created as a benchmark for 3D hand pose
estimation from egocentric thermal image. The goal of this task is estimate the 3D hand joints from egocentric thermal images.  Previous datasets only provide depth, RGB images or both of them as the input spectra, unable to support the study of NIR or thermal image-based 3D hand pose estimation. ThermoHands fills the gap by providing a moderate amount of multi-spectral image data, from infrared to visual light, paired with depth images. Moreover, we capture bimanual actions from both egocentric and exocentric viewpoints and design hand-object as well as hand-virtual interaction actions to facilitate a wide range of applications. 

\noindent\textbf{Who created the dataset (e.g., which team, research group) and on behalf of which entity (e.g., company, institution, organization)?}

This dataset is presented by the MAPS Lab at University of Edinburgh.

\noindent\textbf{Who funded the creation of the dataset?}

This research is partially supported by the Engineering and Physical Sciences Research Council (EPSRC) under the Centre for Doctoral Training in Robotics and Autonomous Systems at the Edinburgh Centre of Robotics (EP/S023208/1), and partially supported by Cisco Research.

\subsection{Composition}
\noindent\textbf{What do the instances that comprise the dataset represent (e.g.,
documents, photos, people, countries)?}

We provide 95,924 samples in our ThermoHands dataset. Each sample consists of the following: 1 egocentric RGB image; 1 egocentric depth image; 1 egocentric NIR image; 1 egocentric thermal image; 1 exocentric RGB image; 1 exocentric depth image. For each sample from the main part (recorded under the normal office scenario), we also include the 3D hand pose ground-truth annotated with our automatic annotation method.

\noindent\textbf{How many instances are there in total (of each type, if appropriate)?} 

There are 95,924 samples in total. For the main part, there are 84,352 samples in total, 47,436 for training, 12,914 for validation and 24,002 for testing. For other settings, there are 3,188 for darkness, 2,508 for sun glare, 3,068 for gloves and 2,808 for kitchen.

\noindent\textbf{Does the dataset contain all possible instances or is it a sample
(not necessarily random) of instances from a larger set?}

The dataset contain all possible instances we collected. 

\noindent\textbf{What data does each instance consist of?}

Each instance consist of exocentric RGB and depth images, egocentric RGB, depth, NIR and thermal images. Each instance from the main part also include the 3D hand pose (joint and mesh) annotations.

\noindent\textbf{Is there a label or target associated with each instance?}

There is a 3D hand joint and a 3D hand mesh label for each instance from the main part.

\noindent\textbf{Is any information missing from individual instances?}

For instances from the auxiliary part, the annotations are missing because our automatic annotation approach becomes infeasible. Specifically, under darkness and glove settings, MeidiaPipe Hands and SAM fails to detect and segment hands on RGB images. Under the sun glare setting, depth images are not as reliable, making our annotation inaccurate. In the kitchen environment, our annotation method suffers from the inter-occlusion of two hands during certain interaction actions (e.g., wash hands, wash mugs).

\noindent\textbf{Are relationships between individual instances made explicit
(e.g., users’ movie ratings, social network links)?}

No. 

\noindent\textbf{Are there recommended data splits (e.g., training, development/validation,
testing)?}

We split the main part of our dataset into the training, validation and testing sets by subjects with a ratio of 4:1:2. We recommend the users following our data splits. 

\noindent\textbf{Are there any errors, sources of noise, or redundancies in the
dataset?}

There exist inevitable errors in our annotations due to the imperfect predictions of off-the-shelf SAM and MediaPipe Hands and our optimization errors. The noises exist in our auxiliary data part, where the RGB images suffer from the darkness while the depth and NIR images are affected by the sun glare.

\noindent\textbf{Is the dataset self-contained, or does it link to or otherwise rely on
external resources (e.g., websites, tweets, other datasets)?}

Our dataset is self-contained.

\noindent\textbf{Does the dataset contain data that might be considered confidential (e.g., data that is protected by legal privilege or by doctor–
patient confidentiality, data that includes the content of individuals’ non-public communications)?}

No. 

\noindent\textbf{Does the dataset contain data that, if viewed directly, might be offensive, insulting, threatening, or might otherwise cause anxiety?}

No.

\noindent\textbf{Does the dataset identify any subpopulations (e.g., by age, gender)?}

No.

\noindent\textbf{Is it possible to identify individuals (i.e., one or more natural persons), either directly or indirectly (i.e., in combination with other
data) from the dataset?}

No. 

\noindent\textbf{Does the dataset contain data that might be considered sensitive
in any way (e.g., data that reveals race or ethnic origins, sexual orientations, religious beliefs, political opinions or union memberships, or locations; financial or health data; biometric or genetic
data; forms of government identification, such as social security
numbers; criminal history)?}

No.

\subsection{Collection Process}
\noindent\textbf{How was the data associated with each instance acquired?}

During capture, our participants are asked to perform pre-defined
hand-object and hand-virtual interaction actions within the playground above the table. Our data was collected using a customized head-mounted sensor platform (HMSP) and an exocentric platform. The annotations for the main part were generated using our automatic labelling approach.

\noindent\textbf{What mechanisms or procedures were used to collect the data
(e.g., hardware apparatuses or sensors, manual human curation,
software programs, software APs)?}

The HMSP consists of three major components: a cushion for comfort, a base component that provides a 30-degree downward tilt, and a sensor board that carries one Intel Realsense L515 LiDAR camera and a Teledyne FLIR Boson 640 long-wave infrared (LWIR) camera. The exocentric platform is built on a tripod mounted with an Intel RealSense D455 RGB-D camera. 

We use a single PC to simultaneously gather data streams from two sensor
platforms, ensuring the synchronization of their timestamps. After collection, we synchronize six
types of images, each with distinct frame rates, w.r.t. the timestamps of thermal images (8.5fps),
thereby generating synchronized multi-spectral, multi-view data samples as our released data

% \textbf{FQ:}
% we can refer to the datasheet at the end of this doc: \href{https://openreview.net/attachment?id=ApqgcSnhjh&name=supplementary_material}{https://openreview.net/attachment?id=ApqgcSnhjh$\&$name=$supplementary_material$}

\noindent\textbf{If the dataset is a sample from a larger set, what was the sampling
strategy (e.g., deterministic, probabilistic with specific sampling
probabilities)?}

The dataset contain all possible instances we collected.

\noindent\textbf{Who was involved in the data collection process (e.g., students,
crowdworkers, contractors) and how were they compensated (e.g.,
how much were crowdworkers paid)?}

Volunteer students were involved in the data collection.  

\noindent\textbf{Over what timeframe was the data collected?}

The collection is conducted between January 2024 and March 2024. We do not provide the timeframes of the data instances.

\noindent\textbf{Were any ethical review processes conducted (e.g., by an institutional review board)?}

The study has been conducted ethical review processed by the ethics review board from the School of Informatics, University of Edinburgh. 

\noindent\textbf{Did you collect the data from the individuals in question directly,
or obtain it via third parties or other sources (e.g., websites)?}

We collect the data directly from our participants in our lab via sensor recording.

\noindent\textbf{Were the individuals in question notified about the data collection?}

Yes, individuals were notified, and participant consent forms were signed before the collection.

\noindent\textbf{Did the individuals in question consent to the collection and use
of their data?}

Yes, consent was obtained from the participants.

\noindent\textbf{If consent was obtained, were the consenting individuals provided with a mechanism to revoke their consent in the future or for certain uses?}

If our participants wish to revoke their consent after finding sensitive data, they can contact us and request to delete or cover the sensitive content from the website hosting our data.

\noindent\textbf{Has an analysis of the potential impact of the dataset and its use
on data subjects (e.g., a data protection impact analysis) been conducted?}

Yes, we conduct an analysis of the potential impact of the dataset and its use on data subjects when submitting our ethics review application.

\subsection{Preprocessing/cleaning/labeling}

\noindent\textbf{Was any preprocessing/cleaning/labeling of the data done (e.g.,
discretization or bucketing, tokenization, part-of-speech tagging,
SIFT feature extraction, removal of instances, processing of missing values)?}

We use our proposed automatic hand pose annotation method to generate the 3D hand joint and mesh ground-truth for the main part. 

\noindent\textbf{Was the “raw” data saved in addition to the preprocessed/cleaned/labeled
data (e.g., to support unanticipated future uses)?}

The "raw" ROS bags were saved on our PC but will not be released.

\noindent\textbf{Is the software that was used to preprocess/clean/label the data
available?}

We will provide the code used to achieve our automatic hand pose annotation.

\subsection{Uses}

\noindent\textbf{Has the dataset been used for any tasks already?}

Yes. We use this dataset to evaluate state-of-the-art methods and our baseline method in this work for 3D hand pose estimation.

\noindent\textbf{Is there a repository that links to any or all papers or systems that
use the dataset?}

No. 

\noindent\textbf{What (other) tasks could the dataset be used for?}

Beside hand pose estimation, this dataset can be used for hand action recognition, cross-modal image synthetics and hand pose forecasting.

\noindent\textbf{Is there anything about the composition of the dataset or the way
it was collected and preprocessed/cleaned/labeled that might impact future uses?}

No.

\noindent\textbf{Are there tasks for which the dataset should not be used?}

The dataset should be solely used for research purposes.

\subsection{Distribution}

\noindent\textbf{Will the dataset be distributed to third parties outside of the entity (e.g., company, institution, organization) on behalf of which
the dataset was created?}

Yes, this dataset will be open-sourced. 

\noindent\textbf{How will the dataset will be distributed (e.g., tarball on website,
API, GitHub)?}

The data will be available on the cloud platform which hosts our dataset. Currently, we upload our dataset to the \href{https://uoe-my.sharepoint.com/personal/s1901843_ed_ac_uk/_layouts/15/onedrive.aspx?id=%2Fpersonal%2Fs1901843%5Fed%5Fac%5Fuk%2FDocuments%2FDatasets%2FThermoHands&ga=1}{Onedrive platform} so that the reviewers can download them for viewing.

\noindent\textbf{When will the dataset be distributed?}

This dataset will be distributed to the public in August 2024.

\noindent\textbf{Will the dataset be distributed under a copyright or other intellectual property (IP) license, and/or under applicable terms of use
(ToU)?}

The ThermoHands dataset is published under MIT license, which means everyone can use this dataset
for non-commercial research purpose.

\noindent\textbf{Have any third parties imposed IP-based or other restrictions on
the data associated with the instances?}

No. 

\noindent\textbf{Do any export controls or other regulatory restrictions apply to
the dataset or to individual instances?}

No. 

\subsection{Maintenance}

\noindent\textbf{Who will be supporting/hosting/maintaining the dataset?}

The authors will be supporting, hosting, and maintaining the dataset.

\noindent\textbf{How can the owner/curator/manager of the dataset be contacted
(e.g., email address)?}

Please contact the corresponding author regarding this dataset. Chris Xiaoxuan Lu: \texttt{xiaoxuan.lu@ucl.ac.uk}.

\noindent\textbf{Is there an erratum?}

No. We will provide the erratum as soon as the need arises.

\noindent\textbf{Will the dataset be updated (e.g., to correct labeling errors, add
new instances, delete instances)?}

We will continue to support ThermoHands dataset to improve annotation accuracy, add new data and provide new labels.

\noindent\textbf{If the dataset relates to people, are there applicable limits on the
retention of the data associated with the instances (e.g., were the
individuals in question told that their data would be retained for
a fixed period of time and then deleted)?}

No.

\noindent\textbf{Will older versions of the dataset continue to be supported/hosted/maintained?}

Yes.

\noindent\textbf{If others want to extend/augment/build on/contribute to the
dataset, is there a mechanism for them to do so?}

Yes, they can directly contact us via email  or raise new issues to ThermoHands github repository: \href{https://github.com/LawrenceZ22/ThermoHands}{https://github.com/LawrenceZ22/ThermoHands}.
