# Supplementary material for: ThermoHands: A Benchmark for 3D Hand Pose Estimation from Egocentric Thermal Images
Source: arXiv:2403.09871 source file (2025-02-27)
Supplement: Supplementary file 2 [file motivation.tex]

\section{Motivation}

The key idea of robust egocentric hand pose estimation seeks to develop methods to determine the 3D positions of 21 joints per hand, catering to the intricate environments encountered in real-world applications. The key to achieve this goal is the development of a hand pose estimator that remains unaffected by the vicissitudes of lighting conditions, particularly in strong light and darkness scenarios. While the prevailing approach in the industry integrates active Near-Infrared (NIR) and RGB cameras to facilitate hand pose estimation under optimal lighting conditions, leveraging NIR cameras in darkness through the emission of NIR light—imperceptible to the human eye—this strategy is not without its flaws. The concurrent operation of multiple active NIR emitters precipitates mutual interference, resulting in significant distortion within NIR imagery. Moreover, the deployment of active NIR emitters incurs additional energy consumption, a critical consideration for mobile mixed-reality (MR) devices.

Compared to imaging in the visible spectrum and NIR spectrum, thermal imaging's unique ability to provide consistent imaging across various lighting conditions—from the brilliance of daylight to the pitch of darkness—positions it as a superior alternative. Its capacity to capture the consistent thermal signature of the human body enables straightforward segmentation of human hands from the surrounding environment, facilitating precise hand pose estimation. Moreover, the nature that all objects above absolute zero emits Long-Wave Infrared (LWIR) radiation eliminates the challenge of shadows that often compromise image fidelity in visible spectrum imaging. This characteristic, coupled with the passive nature of thermal cameras, significantly reduces energy consumption, making it an ideal solution for SLAM in visually degraded environments and advancing the exploration of egocentric thermal imagery for hand pose estimation.

In light of thermal imaging's distinct advantages for egocentric hand pose estimation, its integration into MR devices promises not only a reduction in sensor count and imaging modalities but also a potential decrease in production costs by supplanting the specialized hand tracking apparatuses currently in use. This paradigm shift not only addresses the challenges posed by adverse lighting conditions and obstructive handwear but also aligns with the sustainability and efficiency imperatives of next-generation MR technologies.
