# Supplementary material for: ThermoHands: A Benchmark for 3D Hand Pose Estimation from Egocentric Thermal Images
Source: arXiv:2403.09871 source file (2025-02-27)
Supplement: Supplementary file 3 [file plan.tex]

\newpage
\section{Hosting, Licensing, and Maintenance Plan}

\noindent\textbf{Hosting}

The dataset will be hosted on a cloud platform to ensure accessibility and reliability. The authors of the dataset will be responsible for hosting. This includes setting up and maintaining a valid url to support the dataset's accessibility.

\noindent\textbf{Licensing}

The ThermoHands dataset is published under the MIT license. The MIT license allows for free use, modification, and distribution of the dataset for non-commercial research purposes. This license promotes open access and encourages the research community to utilize and build upon the dataset without significant restrictions. There are no third-party imposed IP-based or other restrictions on the data associated with the instances in the dataset. Additionally, there are no export controls or other regulatory restrictions applicable to the dataset or to individual instances within the dataset.

\noindent\textbf{Maintenance}

The authors will be responsible for the ongoing support, maintenance, and updates of the dataset. This includes addressing any technical issues, ensuring data integrity, and responding to user queries. For any inquiries or support related to the dataset, users can contact the corresponding author, Chris Xiaoxuan Lu, via email at \texttt{xiaoxuan.lu@ucl.ac.uk}. The dataset will be updated periodically to correct any labeling errors, add new instances, and delete any problematic instances. An erratum will be provided as soon as the need arises to ensure users are aware of any corrections or updates. Older versions of the dataset will continue to be supported, hosted, and maintained to ensure that past research relying on earlier versions remains valid. Researchers interested in extending, augmenting, or contributing to the dataset can do so by contacting the authors directly via email or raise issues in our github repository. This open channel encourages collaborative improvements and additions to the dataset.
