# Supplementary material for: ThermoHands: A Benchmark for 3D Hand Pose Estimation from Egocentric Thermal Images
Source: arXiv:2403.09871 source file (2025-02-27)
Supplement: Supplementary file 4 [file accessibility.tex]

\section{Data Accessibility}

\begin{itemize}
    \item Github repository: \href{https://github.com/LawrenceZ22/ThermoHands}{https://github.com/LawrenceZ22/ThermoHands}
    \item Dataset download link: \href{https://uoe-my.sharepoint.com/:f:/g/personal/s1901843_ed_ac_uk/EpgF2qQKonZOtwlStwTwlxwBj6fQNEk6PLsFb_p_HjsmEA}{University of Edinburgh - Onedrive platform} 
    \item Demo video: \url{https://youtu.be/-oXKspAEyhg}.
\end{itemize}
