# Supplementary material for: ThermoHands: A Benchmark for 3D Hand Pose Estimation from Egocentric Thermal Images
Source: arXiv:2403.09871 source file (2025-02-27)
Supplement: Supplementary file 5 [file statement.tex]

\section{Author Statement}
The authors confirm that they bear all responsibility in case of any violation of rights during the
collection of the data or other work, and will take appropriate action when needed, e.g. to remove data
with such issues. The authors also confirm the licenses provided with the data and code associated
with this work.
